# Supplementary material for: Submodular Reinforcement Learning
Source: arXiv:2307.13372 source file (2024-05-24)
Supplement: Supplementary file 1 [file neurips_2023.tex]

\documentclass{article}

% if you need to pass options to natbib, use, e.g.:
\PassOptionsToPackage{numbers, sort,compress}{natbib}
%     \PassOptionsToPackage{numbers, compress}{natbib}
% before loading neurips_2023

% ready for submission
% \usepackage{neurips_2023}

% to compile a preprint version, e.g., for submission to arXiv, add add the
% [preprint] option:
    \usepackage[preprint]{neurips_2023}

% to compile a camera-ready version, add the [final] option, e.g.:
     % \usepackage[final]{neurips_2023}
 % \usepackage[final]{ewrl_2023}

% to avoid loading the natbib package, add option nonatbib:
%    \usepackage[nonatbib]{neurips_2022}
\usepackage[utf8]{inputenc} % allow utf-8 input
\usepackage[T1]{fontenc}    % use 8-bit T1 fonts
\usepackage{hyperref}       % hyperlinks
\usepackage{url}            % simple URL typesetting
\usepackage{booktabs}       % professional-quality tables
\usepackage{amsfonts}       % blackboard math symbols
\usepackage{nicefrac}       % compact symbols for 1/2, etc.
\usepackage{microtype}      % microtypography
\usepackage{xcolor}         % colors
\usepackage{svg}
\usepackage{xspace}
\usepackage[export]{adjustbox}
\usepackage{printlen}
\uselengthunit{cm}
\usepackage{comment}
\usepackage{amsmath}
\usepackage{amsthm}
\usepackage{graphicx}
\usepackage{rotating}
\usepackage{float}
\usepackage{mathrsfs}
\usepackage{amssymb}
\usepackage{autobreak}
\usepackage{mathtools}
\usepackage{wrapfig}
\usepackage{bbm}
\usepackage{algorithm,algcompatible}
\usepackage[permil]{overpic}
\usepackage[noend]{algpseudocode}

\usepackage{subcaption}
\usepackage{lipsum}
\usepackage{outlines}
\usepackage[capitalise]{cleveref}
\usepackage{tikz}
\usetikzlibrary{shapes,backgrounds,patterns}
\usepackage[absolute]{textpos}
\usepackage{thmtools} 
\usepackage{thm-restate}

\usepackage{thmtools} 
\usepackage{thm-restate}
\allowdisplaybreaks
\usepackage[toc,page,header]{appendix}
\usepackage{minitoc}
\usepackage{longtable,xtab,booktabs}
 %,numberwithin=section

 %,numberwithin=section

 %,numberwithin=section

\newsavebox{\algleft}
\newsavebox{\algright}
\newsavebox{\figright}

\algdef{SE}[DOWHILE]{Do}{doWhile}{\algorithmicdo}[1]{\algorithmicwhile\ #1}%

\input{macros}
\allowdisplaybreaks
\makeatletter
\def\thanks#1{\protected@xdef\@thanks{\@thanks
        \protect\footnotetext{#1}}}
\makeatother

\title{Submodular Reinforcement Learning}
% \title{Reinforcement Learning with Submodular Rewards}

% The \author macro works with any number of authors. There are two commands
% used to separate the names and addresses of multiple authors: \And and \AND.
%
% Using \And between authors leaves it to LaTeX to determine where to break the
% lines. Using \AND forces a line break at that point. So, if LaTeX puts 3 of 4
% authors names on the first line, and the last on the second line, try using
% \AND instead of \And before the third author name.

\author{%
  Manish Prajapat\thanks{Code available at \url{https://github.com/manish-pra/non-additive-RL}}  \\
%   ETH AI Center\\
  ETH Zurich\\
  \texttt{manishp@ai.ethz.ch} \\
  % examples of more authors
   \And
   Mojm\'ir Mutn\'y \\
%   Dept. of Computer Science\\
% Department of Computer Science\\
   ETH Zurich \\
   \texttt{mmutny@ethz.ch} \\
   \And
   Melanie N. Zeilinger \\
%   Institute of Dynamic Systems \& Control \\
% IDSC\\
   ETH Zurich \\
   \texttt{mzeilinger@ethz.ch} \\
   \And
   Andreas Krause \\
%   Dept. of Computer Science \\
% Department of Computer Science\\
   ETH Zurich \\
   \texttt{krausea@ethz.ch} \\
  % \And
  % Coauthor \\
  % Affiliation \\
  % Address \\
  % \texttt{email} \\
}

\begin{document}

\maketitle

\input{sections/abstract}

\section{Introduction}
\input{sections/1-introduction}
%motivation - why is this good, and why classical RL cannot solve it. 
%related work 
% \input{sections/1.1-related-work}
\vspace{-1mm}
\section{Submodular RL: Preliminaries and Problem Statement}
\vspace{-1mm}
\label{sec: preliminaries}
\input{sections/2-preliminaries}

\section{Submodular RL: Theoretical Limits}
\label{sec: NP_hard}
\input{sections/3-subrl_analysis}
% introduce the problem - formally 
% state the hardness

% how to transition: In worst case, NP-hard to solve, but still practically solvable as its important. We provide provide geenral alg in the next section and then moving from wors-tscase we provide provable 1/2 approximation in polynomial time for a speicific class of MDPs. 
\input{sections/psuedocode}
\section{General Algorithm: Submodular Policy Optimization \subPOh}
\label{sec: algo}
\input{sections/4-algorithm}
\section{Provable Guarantees in Simplified Settings}
\label{sec: theory}
\input{sections/3.1-Provable_convergence}
% definitoion e-bandit mdp + discsussion 
% statement of the result 
% connection DR-submodualrity 
% FW connection 
\section{Related Work}
\label{sec: related_works}
\input{sections/1.1-related-work}
\vspace{-3 mm}
\section{Experiments}
\vspace{-2 mm}
\label{sec: experiments}
\input{sections/5-experiments}
% 1. grid experiment 
% 2. steiner covering 
% 3. D-experimental design 
% 4. car example (no non-markovian result) 
% 5. mujoco (no non-markovian result) 
\vspace{-2 mm}
\section{Conclusion}
\vspace{-2 mm}
\input{sections/6-conclusion}

\input{sections/acknowledge}

% \section*{References}

\bibliographystyle{unsrtnat} %amsalpha abbrvnat unsrt apalike
\bibliography{ref.bib}

%%%%%%%%%%%%%%%%%%%%%%%%%%%%%%%%%%%%%%%%%%%%%%%%%%%%%%%%%%%%
\newpage
% \section{Supplementary Material}
\appendix
\part{Appendix}
\input{appendix/proposition_proofs}
\newpage
\input{appendix/1-inapproximability}
\newpage
\section{Submodular policy optimization, \subPOh's policy gradient proof}
\input{appendix/PG}
\newpage
\section{Provable Guarantees in Simplified Settings}
\input{appendix/DR-submodularity}
\newpage
\section{Experiments}
\input{appendix/experiments}
% Authors may wish to optionally include extra information (complete proofs, additional experiments and plots) in the appendix. All such materials should be part of the supplemental material (submitted separately) and should NOT be included in the main submission.

\end{document}
